# Supplementary material for: Exploring Autonomous Agentic Data Engineering for Model Specialization
Source: arXiv:2605.30407 source file (2026-08-31)
Supplement: Supplementary file 1 [file human_data_config.tex]

% Across automated settings, we fix the teacher model to Qwen3-30B-A3B. We cap the API budget at 5{,}000 calls for \textit{Iterative Agent}, and use the official \textit{DataFlow} configuration with 6{,}000 calls. Each final synthesized training set contains 2{,}000 examples.
